# Supplementary material for: Adaptive Regularization of Representation Rank as an Implicit Constraint of Bellman Equation
Source: arXiv:2404.12754 source file (2024-04-19)
Supplement: Supplementary file 1 [file Appendix.tex]

\setcounter{section}{0}
\setcounter{equation}{0}

\section{THEORETICAL RESULTS}

\textbf{Lemma 1}(Ensemble Sample Diversity Decomposition) Given the state-action visit distribution of the ensemble policy $\rho$. The entropy of this distribution is $\mathcal{H}(S,A)$. Notice that this term can be decomposed into two parts:\\
\textbf{Proof.}

\begin{equation}
\begin{aligned}
    \mathcal{H}(\rho)&=\mathbb{E}_{(s,a)\sim \rho}[-\log(\rho(s,a))]\\
    &=\mathbb{E}_{(s,a,z)\sim \rho}\left[\log \frac{\rho(s,a|z)}{\rho(s,a)}-\log \rho(s,a|z)\right]\\
    &= \mathbb{E}_{z}\left[\mathcal{D_{KL}}(\rho(s,a|z)||\rho(s,a)) + \mathcal{H}(\rho|z)\right]
\end{aligned}
\end{equation}

\textbf{Lemma 2}\\
\textbf{Proof.}
By definition,
\begin{equation}
    I(\rho;z) = H(\rho) - H(\rho|z) = H(z) - H(z|\rho)
\end{equation}
By randomly selecting the latent variable $z$, we consider that $H(z)$ is a constant depending on the number of $z$. Thus, we have,
\begin{equation}
\begin{aligned}
    H(z|\rho) &= H(z) + H(\rho|z) - H(\rho) \\
             &\propto \mathbb{E}_{(s,a,z)\sim p(s,a,z)}[-\log p(s,a|z)]-\mathbb{E}_{(s,a)\sim p(s,a)}[-\log p(s,a)] \\
             &=\mathbb{E}_{(s,a,z)\sim p(s,a,z)}[-\log p(s,a|z)] - \int -p(s,a)\log p(s,a) dsda  \\
             &=\mathbb{E}_{(s,a,z)\sim p(s,a,z)}[-\log p(s,a|z)] - \int -p(s,a,z)\log p(s,a) dsdadz \\
             &=\mathbb{E}_{(s,a,z)\sim p(s,a,z)}[\log p(s,a)-\log p(s,a|z)] \\
\end{aligned}
\end{equation}
Where, $p(s,a)=\int p(s,a|z)p(z) dz = \frac{1}{n}\sum_{n} p(a|s,z)$. \\
Then, 
\begin{equation}
\begin{aligned}
    H(z|\rho) &= \mathbb{E}_{(s,a,z)\sim p(s,a,z)}[-\log p(z|s,a)]\\
             &= H(z) + H(\rho|z) - H(\rho) \\
             &\propto \mathbb{E}_{(s,a,z)\sim p(s,a,z)}\left[\frac{1}{n}\sum_{n} p(a|s,z)-\log p(a|s,z)\right]
             &\propto -\mathcal{D}_{\mathcal{KL}}\left[p(a|s,z)||\frac{1}{n}\Sigma_{n} p(a|s,z)\right]
\end{aligned}
\end{equation}
\textbf{Lemma 3} Let $X_1, X_2, ..., X_N$ be an infinite sequence of i.i.d. random variables with a probability density function (PDF) of $f(x)$ and a cumulative distribution function (CDF) of $F(x)$. Let $X_{1:N} \leq X_{2:N} \leq X_{3:N} ...\leq X_{N:N}$ be the order statistics corresponding to $\{X_i\}_N$. Denote PDF and CDF of the $k$-th order statistic $X_{k:N}$ as $f_{k:N}$ and $F_{k:N}$ respectively. The following statements hold.\\

(i) $F_{N:N}(x) = (F(x))^N$. $f_{N:N}(x) = Nf(x)(F(x))^{N - 1}$\\

(ii) $F_{1:N}(x) = 1 - (1 - F(x))^N$. $f_{1:N}(x) = Nf(x)(1 - F(x))^{N - 1}$\\

(iii) $\mu - \frac{(N - 1)\sigma}{\sqrt{2N-1}} \leq \mathbb{E}[X_{1:N}] \leq \mu, N>1$. $\mathbb{E}[X_{1:N+1}]\leq\mathbb{E}[X_{1:N}]$\\

(iv) Let $\Bar{X}=\frac{1}{N}\Sigma_{i=1}^{N}X_i$, then, $\mathbb{E}[\Bar{X}]=\mu, Var[\Bar{X}]=\frac{1}{N}\sigma^2$\\

(v) If $X_1, X_2, ..., X_N \sim \mathcal{N}(\mu, \sigma)$, $Var[X_{1:N}]\leq\frac{\sqrt{3}(N-1)}{\sqrt{2N-1}}\sigma^2, N>1. Var[X_{1:N+1}]\geq Var[X_{1:N}]$\\

\textbf{Proof.}

(i) We start from the CDF of $X_{N:N}$. By definition, $F_{N:N}(x) = P(X_{N:N} \leq x)  = P(X_1 \leq x, X_2 \leq x, ..., X_N \leq x)$. Under the assumption of iid. $P(X_1 \leq x, X_2 \leq x, ..., X_N \leq x) = P(X_1 \leq x)P(X_2 \leq x) ... P(X_N \leq x) = (F(x))^N$. The PDF of $X_{N:N}$ can be derived by taking the derivative of PDF. $f_{N:N} = \frac{dF_{N:N}(x)}{dx} = Nf(x)(F(x))^{N - 1}$.\\

(ii) Similar to (i), $F_{1:N}(x) = P(X_{1:N} \leq x) = 1 - P(x \leq X_{1:N}) = P(x \leq X_{})P(x \leq X_1, x \leq X_2, ..., x \leq X_N)$. Under the assumption of iid. $P(x \leq X_1, x \leq X_2, ..., x \leq X_N) = P(X_1 \geq x)P(X_2 \geq x) ... P(X_N \geq x)$. Satisfying the normalization, we have $P(X_1 \geq x)P(X_2 \geq x) ... P(X_N \geq x) = (1 - P(X_1 \leq x))(1 - P(X_2 \leq x))...(1 - P(X_N \leq x)) = (1 - F(x))^N$. Thus, $F_{1:N}(x) = 1 - (1 - F(x))^N$. By taking the derivative of PDF, $f_{1:N}(x) = Nf(x)(1 - F(x))^{N - 1}$.\\

(iii) The detailed proof can be found in \cite{order_statistics}. An brief proof is provided as follows. By definition, 
\begin{equation}
\begin{aligned}
    \mathbb{E}[X_{1:N}] \;\;\; = \;\;\;  &\int^{+\infty}_{-\infty} xf_{1:N}(x)dx \\
                        \;\;\; \overset{(i)}{=}\;\;\; &\int^{+\infty}_{-\infty} xNf(x)(1-F(x))^{N-1}dx\\
                        \overset{u=F(x)}{=} &\int^{1}_{0} x(u)N(1 - u)^{N-1}du\\
\end{aligned}
\end{equation}

To obtain the lower bound on $\mathbb{E}[X_{1:N}]$, we consider the extremum of $\mathbb{E}[X_{1:N}]$ and constrains of mean and variance. For simplification, we consider zero-mean distribution with $\mu=0$ and $\sigma ^2$. The lower bound can be obtained by applying Cauchy-Buniakowsky-Schwarz inequality,
\begin{equation}
    \left( \int^{1}_{0} x(u)N(1 - u)^{N-1}du\right)^2 \leq \int^{1}_{0} x^2 du \int^{1}_{0} (N(1 - u)^{N-1})^2 du=\frac{(N-1)^2}{2N-1}\sigma^2, N>1
\end{equation}
Thus, we have $\mathbb{E}[X_{1:N}]\geq \mu - \frac{N-1}{\sqrt{2N-1}}\sigma$ for distribution with mean and variance of $\mu$ and $\sigma$ respectively. By definition, $\mathbb{E}[X_{1:N+1}]=\mathbb{E}[\min(X_{1:N}, X_{N+1})]\leq\mathbb{E}[X_{1:N}]$

(iv) By definition, 
\begin{equation}
    \mathbb{E}[\Bar{X}] = \mathbb{E}\left[\frac{1}{N}\Sigma_{i=1}^{N}X_i\right] = \frac{1}{N}\Sigma_{i=1}^{N}\mathbb{E}[X_i]=\mu
\end{equation}

\begin{equation}
\begin{aligned}
    Var[\Bar{X}] &= Var\left[\frac{1}{N}\Sigma_{i=1}^{N}X_i\right]\\ 
    &= \mathbb{E}\left[\left(\frac{1}{N}\Sigma_{i=1}^{N}X_i\right)^2\right] - \mathbb{E}^2\left[\frac{1}{N}\Sigma_{i=1}^{N}X_i\right]\\
    &=\frac{1}{N^2}\mathbb{E}\left[\Sigma_{i=1}^{N}\Sigma_{j=1}^{N}X_iX_j \right] - \mu^2\\
    &=\frac{1}{N^2}\mathbb{E}\left[\Sigma_{i=1}^{N}X_i^2\right] + \frac{1}{N^2}\Sigma_{i=1}^N\Sigma_{j=1,j\neq i}^N\mathbb{E}[X_i]\mathbb{E}[X_j] - \mu^2\\
    &= \frac{1}{N}(\mu^2 + \sigma^2) - \frac{1}{N}\mu^2\\
    &= \frac{1}{N}\sigma^2
\end{aligned}
\end{equation}

(v) By definition, 
\begin{equation}
\begin{aligned}
    Var[X_{1:N}] \;\;\; = \;\;\;  &\int^{+\infty}_{-\infty} x^2f_{1:N}(x)dx \\
                        \;\;\; \overset{(i)}{=}\;\;\; &\int^{+\infty}_{-\infty} x^2Nf(x)(1-F(x))^{N-1}dx\\
                        \overset{u=F(x)}{=} &\int^{1}_{0} x^2N(1 - u)^{N-1}du\\
\end{aligned}
\end{equation}
Similarly, The bound can be obtained by applying Cauchy-Buniakowsky-Schwarz inequality.
\begin{equation}
    \left(\int^{1}_{0} x^2N(1 - u)^{N-1}du\right)^2\leq\int^{1}_{0} x^4 du \int^{1}_{0} (N(1 - u)^{N-1})^2 du
\end{equation}
Given $(X_1,X_2,X_3,X_4)$ be a random vector subject to normal distribution with $\mathbb{E}[X_i]=0$, we have
\begin{equation}
    \mathbb{E}[X_1X_2X_3X_4]=\mathbb{E}[X_1X_2]\mathbb{E}[X_3X_4] + \mathbb{E}[X_1X_3]\mathbb{E}[X_2X_4] + \mathbb{E}[X_1X_4]\mathbb{E}[X_2X_3]
\end{equation}
Therefore, we have,
\begin{equation}
    \mathbb{E}[X^4] = 3\mathbb{E}^2[X^2]
\end{equation}

Thus, the upper bound for the $Var[X_{1:N}]$ is given by,
\begin{equation}
    Var[X_{1:N}]\leq\frac{\sqrt{3}(N-1)}{\sqrt{2N-1}}\sigma^2, N>1
\end{equation}

\section{Experimental Details} 
\label{Implementation_details}

\subsection{Implementation and Hyper-parameters}

\label{supp:imple_hyper}
Here, we describe certain implementation details of TEEN.  For our implementation of TEEN, we use a combination of TD3~\cite{TD3} and TEEN, where we construct $N$ TD3 agents based on the released code by the autor (https://github.com/sfujim/TD3). We implement a total of $M=5$ TD3 agents through out our entire experiments. For recurrent optimization mentioned in section 4.2, we set the period of recurrent training to be 50k. We provide explicit parameters used in our algorithm in Table~\ref{tab:parameter_settings}. 

% \begin{table}
% \centering
% \caption{Environment Specific Parameters}
%        \begin{tabular}{l|c|c|c}
%         \toprule
%         Environment      & State Dimensions & Action Dimensions & Reward Scale \\
%         \hline
%         Ant-v3           & 111              & 8           &   5   \\
%         HalfCheetah-v3   & 17               & 6           &   5   \\
%         Hopper-v3        & 11               & 3           &   5   \\
%         Humanoid-v3      & 376              & 17          &   20  \\
%         Pusher-v2        & 23               & 7           &   5   \\
%         Walker2d-v3      & 17               & 6           &   5   \\
%         \bottomrule
%     \end{tabular}
%     \label{tab:environment}  
% \end{table}

\subsection{Reproducing Baselines}
For reproduction of TD3, we use the official implementation ( https://github.com/sfujim/TD3). 
For implementation of SAC, we use the code the author provided and use the parameters the author recommended. We use a single Gaussian distribution and use the environment-dependent reward scaling as described by the authors. For a fair comparison, we apply the version of soft target update and train one iteration per time step. 
\begin{table}[H]
    \centering
    \caption{TEEN Parameters settings}
    \begin{tabular}{l|c}
    \toprule
        Parameter & Value \\
        \hline
        Exploration policy & $\mathcal{N}(0,0.1)$\\
        Weight $\alpha$    & 0.2 \\
        
        Number of sub-policies $N$ & 5 \\
        Number of target values $M$ & 2 \\
        Variance of exploration noise & 0.2 \\
        Random starting exploration time steps & $2.5\times10^4$\\
         Optimizer & Adam\cite{DBLP:conf/iclr/LanPFW20}\\
        Learning rate for actor & $3\times10^{-4}$\\ 
        Learning rate for critic & $3\times10^{-4}$\\
        Replay buffer size & $1\times10^6$\\
        Batch size & 256\\
        Discount $(\gamma)$ & 0.99\\
        Number of hidden layers & 2\\
        Number of hidden units per layer & 256\\
        Activation function & ReLU\\
        Iterations per time step & 1\\
        Target smoothing coefficient $(\eta)$ & $5\times10^{-3}$ \\
        Variance of target policy smoothing & 0.2 \\
        Noise clip range & $[-0.5,0.5]$\\
        Target critic update interval & $2$\\
    \bottomrule    
    \end{tabular}
    
    \label{tab:parameter_settings}
\end{table}

\section{Additional Experimental Results}
\label{supp::add_res}
\subsection{Additional Evaluation} For an additional Evaluation, We conduct experiments on the state-based DMControl~\cite{dmc} suite. We choose TD3~\cite{TD3}, SAC~\cite{SAC}, RND~\cite{RND}, SUNRISE~\cite{sunrise} as our baselines. We perform interactions for 1 million steps in 10 different seeds and evaluate the algorithm over 10 episodes every 5k steps. We evaluate our algorithm in cheetah-run, finger-spin, fish-swim, walker-walk, walker-run. Our results report the mean scores and standard deviations in the 10 seeds. We show the learning curves in Figure~\cite{dmc}
\begin{figure}[H]
    \centering
    \includegraphics[width=0.95\textwidth]{Images/results_plot_sup.pdf}
    \caption{Learning curves for 5 continuous control tasks on DMControl suite. For better visualization, the curves are smoothed uniformly. The bolded line represents the average evaluation over 10 seeds. The shaded region represents the standard deviation of the average evaluation over 10 seeds.}
    \label{fig:dmc}
\end{figure}
